# Supplementary material for: Digital Twin AI: Opportunities and Challenges from Large Language Models to World Models
Source: arXiv:2601.01321 source file (2026-01-04)
Supplement: Supplementary file 1 [file Supplementary.tex]

% remove all table
\begin{table}[h!]
  \centering
  \caption{Physics-Based AI methods.}
  \rowcolors{1}{white}{babyblueeyes!30}
  \resizebox{\textwidth}{!}{
    \begin{tabular}{llllll}
    \toprule
    \textbf{Model} & \textbf{Year}  & \textbf{Conference/Journal} & \textbf{Architecture} & \textbf{Task}  & \textbf{Code} \\
    \midrule
    \href{https://www.pnas.org/doi/full/10.1073/pnas.1517384113}{SINDy}~\cite{brunton2016discovering} & 2016  & PNAS  & Regression & Automatic Modeling, ODEs & \href{https://github.com/dynamicslab/pysindy}{official} \\
    \href{https://arxiv.org/abs/1710.09668}{PDE-Net}~\cite{long2018pde} & 2018  & ICML  & CNN   & PDEs Automatic Modeling, minor prior & \href{https://github.com/ZichaoLong/PDE-Net}{official} \\
    \href{https://www.sciencedirect.com/science/article/pii/S0021999118307125}{PINN}~\cite{raissi2019physics} & 2019  & J. Comput. Phys. & MLP with physics-based loss & PDE solver, Automatic Modeling & \href{https://github.com/maziarraissi/PINNs}{official} \\
    \href{https://arxiv.org/pdf/1912.00873}{VPINN}~\cite{kharazmi2019variational} & 2019  & arXiv & MLP with physics-based loss & PDE solver, varational method & - \\
    \href{https://www.pnas.org/doi/abs/10.1073/pnas.1906995116}{DSINDy}~\cite{champion2019data} & 2019  & PNAS  & Autoencoder & Automatic modeling, parsimonious models & \href{https://github.com/kpchamp/SindyAutoencoders}{official} \\
    \href{https://www.sciencedirect.com/science/article/pii/S0021999119306308}{PDE-Net 2.0}~\cite{long2019pde} & 2019  & J. Comput. Phys. & CNN   & PDEs Automatic modeling, minor prior, time dependent & \href{https://github.com/ZichaoLong/PDE-Net}{official} \\
    \href{https://www.sciencedirect.com/science/article/pii/S0045782520302127}{CPINNs}~\cite{jagtap2020conservative} & 2020  &  CMAME& MLP with physics-based loss & PDE solver, Conservative System & - \\
    \href{https://www.sciencedirect.com/science/article/pii/S0021999119308411}{Adaptive PINNs}~\cite{jagtap2020adaptive} & 2020  & J. Comput. Phys. & CNN with physics-based loss & PDE solver, high convergence rate & - \\
    \href{https://www.sciencedirect.com/science/article/pii/S0045782520304357}{PPINNs}~\cite{meng2020ppinn} & 2020  &  CMAME& MLP with physics-based loss & time dependent, large scale, PDE solver & - \\
    \href{https://link.springer.com/article/10.1007/s10409-021-01148-1}{PINN for fluid}~\cite{cai2021physics} & 2020  & Acta Mechanica Sinica & MLP with physics-based loss & PDE solver, fluid simulation & - \\
    \href{https://www.sciencedirect.com/science/article/pii/S0045782521000773}{PINN for solid}~\cite{haghighat2021physics} & 2020  &  CMAME& MLP with physics-based loss & PDE solver, solid simulation & - \\
    \href{https://www.science.org/doi/10.1126/sciadv.aay2631}{AI Feynman}~\cite{udrescu2020ai} & 2020  & Science Advances & MLP   & Automatic modeling, Physics knowledge, Physics heuristic & \href{https://github.com/SJ001/AI-Feynman}{official} \\
    \href{https://proceedings.neurips.cc/paper_files/paper/2020/hash/c9f2f917078bd2db12f23c3b413d9cba-Abstract.html}{IBGNN}~\cite{cranmer2020discovering} & 2020  & NeurIPS & GNN   & Generalizable physics modeling & \href{https://github.com/MilesCranmer/symbolic_deep_learning}{official} \\
    \href{https://www.sciencedirect.com/science/article/pii/S0021999120307257}{NSFNet}~\cite{jin2021nsfnets} & 2021  & J. Comput. Phys. & MLP with physics-based loss & PDE solver, fluid simulation & - \\
    \href{https://www.science.org/doi/full/10.1126/sciadv.abi8605}{PI-DeepONet}~\cite{wang2021learning} & 2021  & Science Advances & MLP   & Learning Nonlinear Operators, physical constraints & \href{https://github.com/PredictiveIntelligenceLab/Physics-informed-DeepONet}{official} \\
    \href{https://arxiv.org/abs/2010.08895}{FNO}~\cite{li2020fourier} & 2021  & ICLR  & Fourier & Learning Nonlinear Operators, Fourier Domain & \href{https://github.com/zongyi-li/fourier_neural_operator}{official} \\
    \href{https://arxiv.org/abs/2111.13587}{Adaptive FNO}~\cite{guibas2021adaptive} & 2021  & ICLR  & Fourier, Transformer & Learning nonlinear operators, token mixer, Fourier domain & \href{https://github.com/NVlabs/AFNO-transformer}{official} \\
    \href{https://proceedings.neurips.cc/paper/2021/hash/c9e5c2b59d98488fe1070e744041ea0e-Abstract.html}{MWFF}~\cite{gupta2021multiwavelet} & 2021  & NeurIPS & Fourier & Learning Nonlinear Operators, resolution independent solution & \href{https://github.com/gaurav71531/mwt-operator}{official} \\
    \href{https://www.nature.com/articles/s42256-021-00302-5}{DeepONet}~\cite{lu2019deeponet} & 2022  & NMI & MLP   & Learning nonlinear operators, deterministic and stochastic PDEs solver & \href{https://github.com/lululxvi/deeponet}{official} \\
    \href{https://proceedings.neurips.cc/paper_files/paper/2022/hash/948552777302d3abf92415b1d7e9de70-Abstract-Conference.html}{MAD}~\cite{huang2022meta} & 2022  & NeurIPS & Autodecoder with physics-based loss & Unsupervised learning, nonlinear operator & \href{https://gitee.com/mindspore/mindscience/tree/master/MindElec/}{official} \\
    \href{https://proceedings.neurips.cc/paper_files/paper/2023/hash/f3c1951b34f7f55ffaecada7fde6bd5a-Abstract-Conference.html}{CNO}~\cite{raonic2024convolutional} & 2023  & NeurIPS & CNN   & Learning nonlinear operators, Convolution NN & \href{https://github.com/camlab-ethz/ConvolutionalNeuralOperator}{official} \\
    \href{https://www.pnas.org/doi/abs/10.1073/pnas.2310142120}{ICON}~\cite{yang2023context} & 2023  & PNAS  & Transformer & Operator Learning in inference stage & \href{https://github.com/microsoft/in-context-operator-learning}{official} \\
    \href{https://openreview.net/forum?id=ULzyv9M1j5}{T-JSL}~\cite{li2022transformer} & 2023  & ICLR  & Transformer & Automatic modeling, ill-posed problem & \href{https://github.com/AILWQ/Joint_Supervised_Learning_for_SR}{official} \\
    \href{https://proceedings.neurips.cc/paper_files/paper/2023/hash/590daf74f99ee85df3d8c007df9c8187-Abstract-Conference.html}{FactFormer}~\cite{li2024scalable} & 2023  & NeurIPS & Transformer & Computational efficiency, surrogate modeling & \href{https://github.com/BaratiLab/FactFormer}{official} \\
    \href{https://openreview.net/forum?id=EvyYFSxdgB}{DATS}~\cite{toloubidokhtidats} & 2024  & ICLR  & MLP with physics-based loss & PDE solver, meta learning & \href{https://github.com/maryamTolou/DATS_ICLR2024}{official} \\
    \href{https://openreview.net/forum?id=DO2WFXU1Be}{PINNsFormer}~\cite{zhao2023pinnsformer} & 2024  & ICLR  & Transformer with physics-based loss & PDE solver, high accuracy simulation & \href{https://github.com/AdityaLab/pinnsformer}{official} \\
    \href{https://www.sciencedirect.com/science/article/pii/S0021999124004431}{KNO}~\cite{xiong2024koopman} & 2024  & J. Comput. Phys. & Koopman & Light Weight, Interpretable Operator Learning & \href{https://github.com/Koopman-Laboratory/KoopmanLab}{official} \\
    \href{https://www.nature.com/articles/s42256-024-00844-4}{LNO}~\cite{cao2024laplace} & 2024  & NMI & Laplace & Interpretable Operator Learning, System Identification & \href{https://github.com/qianyingcao/Laplace-Neural-Operator}{official} \\
    \href{https://arxiv.org/abs/2402.02366}{Transolver}~\cite{wu2024transolver} & 2024  & ICML  & Transformer & Complex Geometries Operator Learning & \href{https://github.com/thuml/Transolver}{official} \\
    \bottomrule
    \end{tabular}%
    }
  \label{tab:physics}%
\end{table}%

%Table Data Integration Modeling
\begin{table}[htbp]
  \centering
  \caption{Data integration modeling methods.}
  \rowcolors{1}{white}{babyblueeyes!30}
  \resizebox{\textwidth}{!}{
    \begin{tabular}{llllll}
    \toprule
    \textbf{Model} & \textbf{Year}  & \textbf{Conference/Journal} & \textbf{Architecture} & \textbf{Task}  & \textbf{Code} \\
    \midrule
    \href{https://arxiv.org/abs/2201.12086}{BLIP}~\cite{li2022blip} & 2022  & ICML  & VLM   & Vision-language understanding and generation & \href{https://github.com/salesforce/BLIP}{official} \\
    \href{https://arxiv.org/abs/2309.03905}{ImageBind-LLM}~\cite{han2023imagebindllmmultimodalityinstructiontuning} & 2023  & arXiv & MLLM  & Multimodal instruction following & - \\
    \href{https://arxiv.org/abs/2308.16911}{PointLLM}~\cite{xu2023pointllmempoweringlargelanguage} & 2023  & ECCV  & MLLM  & 3D point cloud understanding & \href{https://github.com/OpenRobotLab/PointLLM}{official} \\
    \href{https://arxiv.org/abs/2306.02858}{Video-LLaMA}~\cite{Zhang2023VideoLLaMAAI} & 2023  & EMNLP & MLLM  & Video understanding & \href{https://github.com/DAMO-NLP-SG/Video-LLaMA}{official} \\
    \href{https://arxiv.org/abs/2306.09093}{Macaw-LLM}~\cite{Lyu2023MacawLLMML} & 2023  & arXiv & MLLM  & Multimodal understanding and generation & - \\
    \href{https://arxiv.org/abs/2309.05519}{Next-GPT}~\cite{Wu2023NExTGPTAM} & 2024  & ICML & MLLM  & Multimodal understanding and generation & \href{https://github.com/NExT-GPT/NExT-GPT}{official} \\
    \href{https://arxiv.org/abs/2301.12597}{BLIP-2}~\cite{Li2023BLIP2BL} & 2023  & ICML  & VLM   & Vision-Language Task & \href{https://github.com/salesforce/BLIP}{official} \\
    \href{https://llava-vl.github.io/}{LLaVA}~\cite{Liu2023VisualIT} & 2023  & NeurIPS & MLLM  & Vision-Language Task & \href{https://llava-vl.github.io/}{official} \\
    \href{https://arxiv.org/abs/2303.17760}{CAMEL}~\cite{li2023camelcommunicativeagentsmind} & 2023  & NeurIPS & Multi-agent & Multi-agent cooperation and interaction & \href{https://github.com/camel-ai/camel}{official} \\
    \href{https://arxiv.org/abs/2308.08155}{AutoGEN}~\cite{wu2023autogenenablingnextgenllm} & 2023  & COLM  & Multi-agent & Multi-agent cooperation and interaction & \href{https://github.com/microsoft/AutoGen}{official} \\
    \href{https://arxiv.org/abs/2308.00352}{MetaGPT}~\cite{hong2023metagptmetaprogrammingmultiagent} & 2023  & ICLR  & Multi-agent & Multi-agent collaboration in complex tasks & \href{https://github.com/meta-gpt/meta-gpt}{official} \\
    \href{https://github.com/DCDmllm/WorldGPT}{WorldGPT}~\cite{ge2024worldgpt} & 2024  & MM & MLLM  & Multimodal world modeling & \href{https://github.com/DCDmllm/WorldGPT}{official} \\
    \href{https://arxiv.org/abs/2403.01133}{TimeAnnotator}~\cite{hota2024evaluating} & 2024  & arXiv & LLM   & Time-series data annotation & - \\
    \href{https://arxiv.org/abs/2401.06866}{Health-LLM}~\cite{kim2024health} & 2024  & arXiv & LLM   & Health prediction & \href{https://github.com/mitmedialab/Health-LLM}{official} \\
    \href{https://arxiv.org/abs/2405.02957}{Agent Hospital}~\cite{li2024agenthospitalsimulacrumhospital} & 2024  & arXiv & LLM   & Medical agent evolution and hospital simulation & - \\
    \href{https://arxiv.org/abs/2406.04692}{Mixture-of-Agents (MoA)}~\cite{wang2024mixtureofagentsenhanceslargelanguage} & 2024  & arXiv & Multi-agent & Natural language understanding and generation & \href{https://github.com/togethercomputer/MoA}{official} \\
    \href{https://arxiv.org/abs/2405.15793}{SWE-agent}~\cite{jimenez2024swebenchlanguagemodelsresolve} & 2024  & arXiv & LLM   & Automated software engineering & \href{https://github.com/princeton-nlp/SWE-agent}{official} \\
    \href{https://arxiv.org/abs/2312.01059}{Swarm-GPT}~\cite{jiao2023swarmgptcombininglargelanguage} & 2024  & ICML  & Multi-agent & Robot choreography design & - \\
    \bottomrule
    \end{tabular}%
    }
  \label{tab:integration}%
\end{table}

% Table Simulation Modeling with Generative AI
\begin{table}[htbp]
  \centering
  \caption{Simulation modeling with generative AI methods.}
  \rowcolors{1}{white}{babyblueeyes!30}
  \resizebox{\textwidth}{!}{
    \begin{tabular}{llllll}
    \toprule
    \textbf{Model} & \textbf{Year}  & \textbf{Conference/Journal} & \textbf{Architecture} & \textbf{Task}  & \textbf{Code} \\
    \midrule
     \href{https://arxiv.org/abs/1812.02784}{StoryGAN}~\cite{1812.02784v2} & 2019  & AAAI  & Sequential Conditional GAN & Story visualization & \href{https://github.com/yitong91/StoryGAN}{official} \\
    \href{https://arxiv.org/abs/2104.10157}{VideoGPT}~\cite{2104.10157v2} & 2021  & arXiv & VQ-VAE and Transformers & Video generation & \href{https://wilson1yan.github.io/videogpt/index.html}{official} \\
    \href{https://arxiv.org/abs/2111.14643}{URF}~\cite{2111.14643v1} & 2021  & CVPR  & Neural Radiance Fields (NeRF) & 3D reconstruction and novel view synthesis & - \\
    \href{https://arxiv.org/abs/2008.02268}{NeRF-W}~\cite{2008.02268v3} & 2021  & CVPR  & Neural Radiance Fields (NeRF) & 3D scene reconstruction and novel view synthesis & \href{https://github.com/bmild/nerf}{official} \\
    \href{https://arxiv.org/abs/2210.02303}{Imagen Video}~\cite{2210.02303v1} & 2022  & arXiv     & Cascade of video diffusion models & Text-to-video generation & \href{https://imagen.research.google/video}{official} \\
    \href{https://arxiv.org/abs/2205.15868}{CogVideo}~\cite{2205.15868v1} & 2022  & ICLR  & 9B-parameter transformer & Text-to-video generation & \href{https://github.com/THUDM/CogVideo}{official} \\
    \href{https://arxiv.org/abs/2202.05263}{Block-NeRF}~\cite{2202.05263v1} & 2022  & arXiv & Neural Radiance Fields (NeRF) & Neural view synthesis & \href{https://waymo.com/research/block-nerf}{official} \\
    \href{https://arxiv.org/abs/2203.09517}{TensoRF}~\cite{2203.09517v2} & 2022  & arXiv & Tensorial Radiance Fields & 3D scene reconstruction and novel view synthesis & \href{https://apchenstu.github.io/TensoRF/}{official} \\
    \href{https://arxiv.org/abs/2112.05504}{BungeeNeRF}~\cite{2112.05504v4} & 2022  & arXiv & Progressive neural radiance field & Multi-scale 3D scene rendering & - \\
    \href{https://arxiv.org/abs/2311.15127}{Stable Video Diffusion}~\cite{2311.15127v1} & 2023  & arXiv & Latent Video Diffusion Model & Text-to-video and image-to-video generation & \href{https://github.com/Stability-AI/generative-models}{official} \\
    \href{https://arxiv.org/abs/2212.05199}{MAGVIT}~\cite{2212.05199v2} & 2023  & CVPR  & Masked Generative Video Transformer & Video generation & \href{https://magvit.cs.cmu.edu}{official} \\
    \href{https://arxiv.org/abs/2309.15103}{LaVie}~\cite{2309.15103v2} & 2023  & arXiv      & Cascaded Latent Diffusion Models & Text-to-video generation & \href{https://vchitect.github.io/LaVie-project/}{official} \\
    \href{https://arxiv.org/abs/2304.08818}{Video LDM}~\cite{2304.08818v2} & 2023  & CVPR  & Latent Diffusion Models & High-resolution video synthesis & \href{https://research.nvidia.com/labs/toronto-ai/VideoLDM/}{official} \\
    \href{https://arxiv.org/abs/2301.10241}{K-Planes}~\cite{2301.10241v2} & 2023  & arXiv & Explicit Radiance Fields & Dynamic scene reconstruction & \href{https://sarafridov.github.io/K-Planes}{official} \\
    \href{https://arxiv.org/abs/2303.14536}{SUDS}~\cite{2303.14536v1} & 2023  & CVPR  & Multi-branch hash table representation & Novel-view synthesis & - \\
    \href{https://arxiv.org/abs/2309.13101}{Deformable 3D Gaussians}~\cite{2309.13101v2} & 2023  & arXiv & Deformable 3D Gaussians Splatting & Monocular dynamic scene reconstruction & \href{https://github.com/ingra14m/Deformable-3D-Gaussians}{official} \\
    \href{https://arxiv.org/abs/2312.00112}{DynMF}~\cite{2312.00112v1} & 2023  & ECCV  & Neural Motion Factorization & Dynamic view synthesis & \href{https://agelosk.github.io/dynmf/}{official} \\
    \href{https://arxiv.org/abs/2312.04557}{GenTron}~\cite{2312.04557v2} & 2024  & CVPR  & Transformer-based diffusion model & Text-to-image and text-to-video generation & \href{https://www.shoufachen.com/gentron_website/}{official} \\
    \href{https://arxiv.org/abs/2310.12190}{DynamiCrafter}~\cite{2310.12190v2} & 2024  & ECCV     & Dual-stream image injection paradigm & Image animation & \href{https://doubiiu.github.io/projects/DynamiCrafter}{official} \\
    \href{https://arxiv.org/abs/2404.05014}{MagicTime}~\cite{2404.05014v1} & 2024  & arXiv     & U-Net & Text-to-video generation & \href{https://github.com/PKU-YuanGroup/MagicTime}{official} \\
    \href{https://arxiv.org/abs/2408.06072}{CogVideoX}~\cite{2408.06072v1} & 2024  & arXiv & 3D Variational Autoencoder & Text-to-video generation & \href{https://github.com/THUDM/CogVideo}{official} \\
    \href{https://arxiv.org/abs/2401.03048}{Latte}~\cite{2401.03048v1} & 2024  & arXiv & Latent Diffusion Transformer & Video Generation & \href{https://maxin-cn.github.io/latte_project}{official} \\
    \href{https://arxiv.org/abs/2310.06114}{UniSim}~\cite{2310.06114v2} & 2024  & arXiv & Video diffusion model & Video captioning & \href{https://universal-simulator.github.io}{official} \\
    \href{https://arxiv.org/abs/2403.14773}{StreamingT2V}~\cite{2403.14773v1} & 2024  & arXiv  &Diffusion Model& Text-to-video generation & \href{https://github.com/Picsart-AI-Research/StreamingT2V}{official} \\
    \href{https://arxiv.org/abs/2310.05737}{MAGVIT-v2}~\cite{2310.05737v3} & 2024  & ICLR  & Masked Language Model & Video generation & \href{https://magvit.cs.cmu.edu/v2}{official} \\
    \href{https://arxiv.org/abs/2312.14125}{VideoPoet}~\cite{2312.14125v4} & 2024  & PMLR     & Decoder-only transformer & Zero-shot video generation & \href{https://sites.research.google/videopoet/}{official} \\
    \href{https://arxiv.org/abs/2402.14797}{Snap Video}~\cite{2402.14797v1} & 2024  & arXiv & Scaled Spatiotemporal Transformers & Text-to-video synthesis & \href{https://snap-research.github.io/snapvideo}{official} \\
    \href{https://arxiv.org/abs/2303.14897}{Seer}~\cite{2303.14897v3} & 2024  & arXiv & Inflated 3D U-Net & Text-conditioned video prediction & - \\
    \href{https://arxiv.org/abs/2401.09047}{VideoCrafter2}~\cite{2401.09047v1} & 2024  & arXiv & Video Diffusion Models & Text-to-video generation & \href{https://github.com/AILab-CVC/VideoCrafter}{official} \\
    \href{https://arxiv.org/abs/2401.09985}{WorldDreamer}~\cite{2401.09985v1} & 2024  & arXiv & Spatial Temporal Patchwise Transformer & Text-to-video, image-to-video synthesis & \href{https://world-dreamer.github.io}{official} \\
    \href{https://arxiv.org/abs/2408.14837}{GameNGen}~\cite{2408.14837v1} & 2024  & arXiv     & Generative Diffusion Model & Interactive World Simulation & \href{https://gamengen.github.io}{official} \\
    \href{https://arxiv.org/abs/2403.12839}{GF-NeRF}~\cite{2403.12839v1} & 2024  & arXiv & Two-stage architecture & Large-scale scene rendering & \href{https://shaomq2187.github.io/GF-NeRF/}{official} \\
    \href{https://arxiv.org/abs/2404.01133}{CityGS}~\cite{2404.01133v3} & 2024  & arXiv & 3D Gaussian Splatting & Large-scale scene reconstruction & \href{https://dekuliutesla.github.io/citygs/}{official} \\
    \href{https://arxiv.org/abs/2310.10642}{4DGS}~\cite{2310.10642v3} & 2024  & ICLR  & 4D Gaussian Splatting & Dynamic novel view synthesis & \href{https://fudan-zvg.github.io/4d-gaussian-splatting}{official} \\
    \href{https://arxiv.org/abs/2401.01339}{Street Gaussians}~\cite{2401.01339v3} & 2024  & arXiv & Explicit scene representation & Dynamic urban street modeling & - \\
    \href{https://arxiv.org/abs/2404.00168}{ML-NSG}~\cite{2404.00168v1} & 2024  & CVPR  & Multi-Level Neural Scene Graph & Novel View Synthesis & \href{https://tobiasfshr.github.io/pub/ml-nsg/}{official} \\
    \href{https://arxiv.org/abs/2501.03575}{Cosmos}~\cite{agarwal2025cosmos} & 2025  & arXiv  & Transformer-based diffusion models and autoregressive models
 & General world simulation, video generation
 & \href{https://github.com/NVIDIA/Cosmos?tab=readme-ov-file}{official} \\
    \href{https://deepmind.google/discover/blog/genie-2-a-large-scale-foundation-world-model/}{Genie 2}~\cite{parker-holder2024genie2} & 2024  & Blog & Autoregressive latent diffusion model & 3D world generation and simulation & \href{https://deepmind.google/discover/blog/genie-2-a-large-scale-foundation-world-model/}{official} \\
    \bottomrule
    \end{tabular}%
    }
  \label{tab:generation}%
\end{table}

% Table Prediction and Decision Making
\begin{table}[htbp]
  \centering
  \caption{Prediction and decision-making methods.}
  \rowcolors{1}{white}{babyblueeyes!30}
  \resizebox{\textwidth}{!}{
    \begin{tabular}{llllll}
    \toprule
    \textbf{Model} & \textbf{Year}  & \textbf{Conference/Journal} & \textbf{Architecture} & \textbf{Task}  & \textbf{Code} \\
    \midrule
    \href{https://www.sciencedirect.com/science/article/pii/S0736584519306660?via\%3Dihub}{DT-HPM}~\cite{Luo2020ah} & 2020  & RCIM  & Hybrid model & Predictive maintenance of CNC machine tools. & - \\
    \href{https://link.springer.com/chapter/10.1007/978-3-030-47638-0_6}{SHM-DT}~\cite{Zhu2020rea} & 2020  & MVUQ  & SHM-DT & Real-time updating of digital twins in structural health monitoring & - \\
    \href{https://onlinelibrary.wiley.com/doi/full/10.1111/tgis.12644}{Traffic Transformer}~\cite{cai2020traffic} & 2020  & TGIS  & Transformer, GCN & Traffic forecasting & \href{https://github.com/tensorflow/models/tree/master/official/transformer}{official} \\
    \href{https://ieeexplore.ieee.org/document/8984243}{PRT-DT}~\cite{Milton2020con} & 2020  & TPEL  & PCE   & Diagnostic analysis of power electronic converters & - \\
    \href{https://ieeexplore.ieee.org/document/9438560}{ATTAIN}~\cite{Xu2021dig} & 2021  & ICST  & GAN, GCN-LSTM & Anomaly detection in cyber-physical systems. & - \\
    \href{https://www.sciencedirect.com/science/article/pii/S0925231220318191}{MDCGCN}~\cite{Li2021tra} & 2021  & Neurocomputing & GCN   & Traffic flow prediction. & - \\
    \href{https://ieeexplore.ieee.org/document/9320532}{DTHS}~\cite{elayan2021digital} & 2021  & IEEE IoT & LSTM, CNN & Real-time health status monitoring and anomaly detection in ECG data & - \\
    \href{https://www.sciencedirect.com/science/article/pii/S0951832021003975}{HAGCN}~\cite{Li2021hie} & 2021  & RESS  & LSTM, GCN & Remaining useful life (RUL) prediction for machinery & - \\
    \href{https://ieeexplore.ieee.org/document/10130979}{ADDT}~\cite{Li2022ano} & 2022  & ISCTech & Transformer-based & Anomaly detection of Internet service quality degradation. & - \\
    \href{https://www.sciencedirect.com/science/article/pii/S2352710222013699}{AID-FS}~\cite{Zhang2022bui} & 2022  & JOBE  & Conv-LSTM & Real-time identification and management of fire scenarios in buildings. & - \\
    \href{https://dl.acm.org/doi/abs/10.1145/3570349}{PhysiQ}~\cite{Wang2022phy} & 2022  & IMWUT & CNN, LSTM & Off-site quality assessment of physical therapy exercises & - \\
    \href{https://ieeexplore.ieee.org/document/9695321}{GITA}~\cite{Wu2022ind} & 2022  & TII   & LSTM  & Indoor tracking for factory logistics & - \\
    \href{https://www.researchsquare.com/article/rs-1730668/v1}{TSTNet}~\cite{Pan2022tem} & 2022  & IJCARS & Transformer, LSTM & Workflow recognition of surgical video & - \\
    \href{https://doi.org/10.1109/ACCESS.2022.3193941}{RTERS}~\cite{subramanian2022digital} & 2022  & IEEE Access & Gradient Boosting & Emotion recognition for personalized healthcare & - \\
    \href{https://ieeexplore.ieee.org/document/9422209}{SuperGraph}~\cite{Yang2022sup} & 2022  & TIE   & GCN   & Rotating machinery fault diagnosis & \href{https://github.com/ChaoyingYang/SuperGraph}{official} \\
    \href{https://www.mdpi.com/2076-3417/13/3/1891}{MTAD-GAN}~\cite{Lian2023ano} & 2023  & Applied Sciences & GAN, LSTM & Anomaly detection in multivariate time series data for oil and gas stations. & - \\
    \href{https://ieeexplore.ieee.org/document/9424948}{SARIMA-LSTM}~\cite{Hao2021hyb} & 2023  & TASE  & SARIMA, LSTM & Real-time anomaly detection in industrial cyber-physical systems (ICPS). & - \\
    \href{https://ieeexplore.ieee.org/document/9733959}{STAR}~\cite{Liang2023spa} & 2023  & TITS  & GCN   & Data recovery in cooperative-intelligent transportation systems (C-ITS). & - \\
    \href{https://www.sciencedirect.com/science/article/pii/S0950705122012849?via\%3Dihub}{DGCRIN}~\cite{Kong2022dyn} & 2023  & KBS   & GCN   & Missing data imputation in spatiotemporal traffic data & - \\
    \href{https://www.sciencedirect.com/science/article/pii/S2352710223015966?via\%3Dihub}{EDTS}~\cite{ding2023intelligent} & 2023  & JoBE  & CNN   & Fire evacuation monitoring and evacuee tracking & - \\
    \href{https://doi.org/10.1016/j.est.2023.107203}{LSTM-DT}~\cite{Yi2023dig} & 2023  & JoES  & LSTM  & Real-time temperature prediction and degradation analysis of lithium-ion batteries & - \\
    \href{https://ieeexplore.ieee.org/document/9779929}{MSTGNN}~\cite{Zhang2023fau} & 2023  & TII   & GNN   & Fault prediction for electromechanical equipment & - \\
    \href{https://www.sciencedirect.com/science/article/pii/S0926580523005009}{AUTCON}~\cite{Zhang2024dig} & 2024  & AUTCON & GCN-LSTM & Real-time monitoring and advanced control of TBM operation & - \\
    \href{https://doi.org/10.1016/j.energy.2023.129681}{DT-LB}~\cite{Li2023enh} & 2024  & Energy & CNN, LSTM & Real-time degradation prediction of lithium-ion batteries & - \\
    \bottomrule
    \end{tabular}%
    }
  \label{tab:prediction-decision}%
\end{table}

% Table Anomaly Detection
\begin{table}[htbp]
  \centering
  \caption{Anomaly detection methods.}
  \rowcolors{1}{white}{babyblueeyes!30}
  \resizebox{\textwidth}{!}{
    \begin{tabular}{llllll}
    \toprule
    \textbf{Model} & \textbf{Year}  & \textbf{Conference/Journal} & \textbf{Architecture} & \textbf{Task}  & \textbf{Code} \\
    \midrule
    \href{https://www.sciencedirect.com/science/article/pii/S0925231215014149}{FaultDiagnosis-SVM}~\cite{Yin2016rec} & 2016  & Neurocomputing & SVM   & Fault diagnosis and process monitoring & - \\
    \href{https://ieeexplore.ieee.org/document/7911887}{LSTM-CPS}~\cite{Goh2017ano} & 2017  & ISHASE & LSTM  & Anomaly detection in cyber-physical systems (CPS) & - \\
    \href{https://ieeexplore.ieee.org/document/8417863}{AD-V2IC}~\cite{russo2018anomaly} & 2018  & VTC   & LSTM, MLP & Anomaly detection in vehicular communications & - \\
    \href{https://www.cambridge.org/core/journals/ai-edam/article/hidden-markov-modelbased-digital-twin-construction-for-futuristic-manufacturing-systems/28B4EBEE42ACB043202A6ED19B96564B}{HMM-DTFMS}~\cite{Ghosh2019hid} & 2019  & AIEDAM & HMM   & Digital twin construction for manufacturing systems & - \\
    \href{https://ieeexplore.ieee.org/document/8598879}{DFDD}~\cite{Xu2019ad} & 2019  & IEEE Access & DNN   & Fault diagnosis in smart manufacturing & - \\
    \href{https://ieeexplore.ieee.org/document/8416777}{FD-wkNN}~\cite{Zhang2019fau} & 2019  & TSM   & kNN   & Fault detection in semiconductor manufacturing processes & - \\
    \href{https://ieeexplore.ieee.org/document/8662186}{CyberAnomalyLR}~\cite{noureen2019anomaly} & 2019  & TPEC  & Logistic Regression & Anomaly detection in cyber-physical systems & - \\
    \href{https://ieeexplore.ieee.org/document/9179030}{SAE-DT}~\cite{Castellani2020rea} & 2021  & TII   & Autoencoder & Anomaly detection in industrial monitoring systems & - \\
    \href{https://www.sciencedirect.com/science/article/pii/S0278612520301151}{HealthDT-B}~\cite{Yu2020ad} & 2021  & JMS   & Bayesian Network & Health monitoring in complex systems & - \\
    \href{https://ieeexplore.ieee.org/document/9449682}{SGDT}~\cite{Danilczyk2021sma} & 2021  & NAPS  & CNN   & Anomaly detection in smart grids & - \\
    \href{https://ieeexplore.ieee.org/document/9712649}{DSC-HMM}~\cite{Wang2022rea} & 2022  & TNSM  & GAN   & Root cause analysis for anomalies in NFV environment & - \\
    \href{https://ieeexplore.ieee.org/document/9816882}{AdaN}~\cite{Shetve2022ada} & 2022  & ICPS  & DBSCAN, Isolation Forest & Real-time anomaly detection in smart manufacturing & - \\
    \href{https://www.mdpi.com/1424-8220/22/4/1430}{MDT-BN}~\cite{Ademujimi2022dig} & 2022  & Sensors & Bayesian Network & Fault diagnostics in manufacturing systems & - \\
    \href{https://ieeexplore.ieee.org/abstract/document/9669046}{AL-DNN}~\cite{Lv2023saf} & 2023  & TII   & DNN   & Fault diagnosis in manufacturing equipment & - \\
    \href{https://ieeexplore.ieee.org/document/10296852}{DRGCN}~\cite{Darvishi2023dee} & 2023  & IEEE Sens. J. & GCN, RNN & Sensor fault detection, isolation, and accommodation in IoT networks & - \\
    \href{https://ieeexplore.ieee.org/document/10122519}{WGAN-DT}~\cite{Hasan2023was} & 2023  & IEEE Sens. J. & WGAN, GAF & Early drift fault detection in wireless sensor networks & - \\
    \href{https://ieeexplore.ieee.org/document/10236947}{MOCAE}~\cite{Hu2023am} & 2023  & JSAC  & Autoencoder & Bearing fault diagnosis & - \\
    \href{https://ieeexplore.ieee.org/document/9927243}{CNN-BDT}~\cite{Wu2023ad} & 2023  & JRFI  & CNN   & Fault diagnosis for bogies of high-speed trains & - \\
    \href{https://www.researchgate.net/publication/370894946_Towards_a_Digital_Twin_in_Human_Brain_Brain_Tumor_Detection_Using_K-Means}{BrainTumorDT}~\cite{Sarris2023tow} & 2023  & MIE   & K-Means & Brain tumor detection & - \\
    \href{https://ieeexplore.ieee.org/document/10239395}{ParkinsonDTHS}~\cite{Abirami2023dig} & 2023  & IEEE Access & kNN   & Parkinson's disease identification and diagnosis & - \\
    \href{https://ieeexplore.ieee.org/stamp/stamp.jsp?arnumber=10234596}{WDT-B}~\cite{Ruah2022ab} & 2023  & JSAC  & Bayesian Model, Multi-agent & Control, monitoring, and data collection in wireless systems & - \\
    \href{https://ieeexplore.ieee.org/document/9999272}{ADDAM}~\cite{Li2023an} & 2023  & TII   & CNN   & Anomaly detection in industrial control systems & - \\
    \bottomrule
    \end{tabular}%
    }
  \label{tab:anomaly}%
\end{table}

% Table Optimization and Control
\begin{table}[htbp]
  \centering
  \caption{Optimization and control methods.}
  \rowcolors{1}{white}{babyblueeyes!30}
  \resizebox{\textwidth}{!}{
    \begin{tabular}{llllll}
    \toprule
    \textbf{Model} & \textbf{Year}  & \textbf{Conference/Journal} & \textbf{Architecture} & \textbf{Task}  & \textbf{Code} \\
    \midrule
    \href{https://ieeexplore.ieee.org/stamp/stamp.jsp?tp=\&arnumber=9211946}{DTRL-planning}~\cite{muller2020dynamic} & 2020  & IEEE Int. Conf. ETFA & DQN   & Planning strategy generation & - \\
    \href{https://ieeexplore.ieee.org/stamp/stamp.jsp?tp=\&arnumber=9303438}{DTACS}~\cite{wang2020adaptive} & 2020  & IEEE Trans. Autom. Sci. Eng. & DQN   & Conveyor systems optimization & - \\
    \href{https://www.sciencedirect.com/science/article/pii/S0098135420305500}{RL-RTO}~\cite{powell2020real} & 2020  & Chemical Engineering Journal & Actor Critic Network & Real-time optimization, chemical reactor & - \\
    \href{https://www.sciencedirect.com/science/article/pii/S0098135421000582}{AC-RL}~\cite{oh2021actor} & 2021  & J. Process Control & DQN   & Real-time optimization, chemical reactor & - \\
    \href{https://arxiv.org/abs/2105.12847}{RDT-AC}~\cite{kafkes2021developing} & 2021  & arXiv & DQN   & Control accelerator & - \\
    \href{https://arxiv.org/abs/1904.04152}{RL-ENMPC}~\cite{gros2019data} & 2021  & IEEE Trans. Autom. Control & DQN   & Computational efficiency control & - \\
    \href{https://www.sciencedirect.com/science/article/pii/S1474034621002202}{DTSR}~\cite{liu2022digital} & 2022  & Advanced Engineering Informatics & GRNN  & Parameter control & - \\
    \href{https://www.sciencedirect.com/science/article/pii/S0038092X23000063}{DT-mincost}~\cite{pan2023real} & 2023  & Solar Energy & DQN   & Cost reduction, solar energy system & - \\
    \href{https://www.sciencedirect.com/science/article/pii/S187775032400214X}{DT}~\cite{schena2024reinforcement} & 2023  & J. Comput. Sci. & DDPG  & RL training & - \\
    \href{https://journalofcloudcomputing.springeropen.com/articles/10.1186/s13677-024-00683-z}{DTRL-scheduling}~\cite{qi2024real} & 2024  & J. Cloud Comput. & DQN   & Cost reduction, power grid system & - \\
    \href{https://www.sciencedirect.com/science/article/pii/S2452414X2400089X}{DTFL}~\cite{yang2024adaptive} & 2024  & J. Ind. Inf. Integr. & Federated learning & Cost reduction, logistic system & - \\
    \href{https://www.sciencedirect.com/science/article/pii/S0009250924002902}{fed-batch RL}~\cite{li2024ai} & 2024  & Chemical Engineering Science & DQN   & Biopharmaceutical process optimization & - \\
    \href{https://arxiv.org/abs/2403.15067}{TD3}~\cite{olayemi2024twin} & 2024  & arXiv & TD3   & Navigate ground vehicle & - \\
    \href{https://arxiv.org/html/2403.13090v1}{DTRL-SIOT}~\cite{sun2024digital} & 2024  & arXiv & DQN   & Control strategy, robot control & - \\
    \bottomrule
    \end{tabular}%
    }
  \label{tab:optimization}%
\end{table}
